# Supplementary material for: Generative Escher Meshes
Source: arXiv:2309.14564 source file (2024-06-17)
Supplement: Supplementary file 1 [file comparison_supp.tex]

\begin{figure}[h]
    \centering
    \captionsetup{justification=centering}
        % \subfloat[]{
        %    \raisebox{0.75in}{\rotatebox[origin=t]{90}{{Ours}}}
        % } 
        \begin{subfigure}[t]{0.45\linewidth}
        \includegraphics[width=\linewidth]{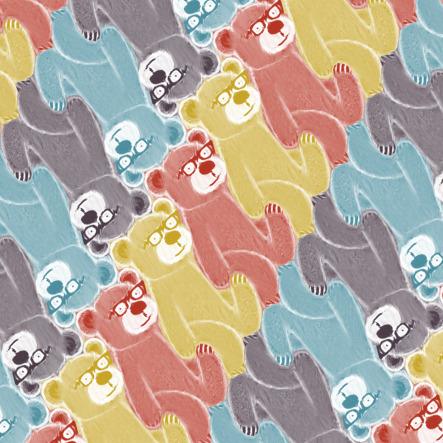}
        \caption{\theprompt{A nerdy bear}}
        \end{subfigure}
        % \begin{subfigure}[t]{0.45\linewidth}
        % \includegraphics[width=\linewidth]{figures/gallery_2/14.jpg}
        % \caption{\theprompt{A penguin}}
        % \end{subfigure}
        \begin{subfigure}[t]{0.45\linewidth}
        \includegraphics[width=\linewidth]{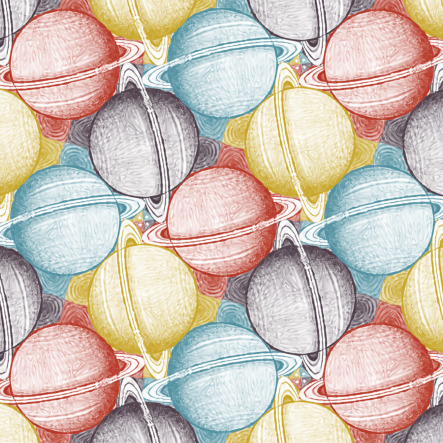}
        \caption{\theprompt{Saturn with shooting stars}}
        \end{subfigure}
        % \begin{subfigure}[t]{0.45\linewidth}
        % \includegraphics[width=\linewidth]{figures/gallery_1/20.jpg}
        % \caption{\theprompt{A lion}}
        % \end{subfigure}
        % \begin{subfigure}[t]{0.45\linewidth}
        % \includegraphics[width=\linewidth]{figures/gallery_2/19.jpg}
        % \caption{\theprompt{A bat}}
        % \end{subfigure}
\\
        % \subfloat[]{
        %    \raisebox{0.75in}{\rotatebox[origin=t]{90}{{Baseline 1}}}
        % } 
        \begin{subfigure}[t]{0.45\linewidth}
        \includegraphics[width=\linewidth]{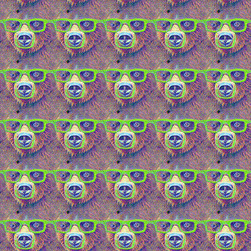}
        \caption{\theprompt{A nerdy bear}}
        \end{subfigure}
        % \begin{subfigure}[t]{0.45\linewidth}
        % \includegraphics[width=\linewidth]{figures/comparison/media_images_010.jpg}
        % \caption{\theprompt{A penguin}}
        % \end{subfigure}
        \begin{subfigure}[t]{0.45\linewidth}
        \includegraphics[width=\linewidth]{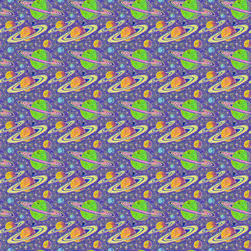}
        \caption{\theprompt{Saturn with shooting stars}}
        \end{subfigure}
        % \begin{subfigure}[t]{0.45\linewidth}
        % \includegraphics[width=\linewidth]{figures/comparison/media_images_012.jpg}
        % \caption{\theprompt{A lion}}
        % \end{subfigure}
        % \begin{subfigure}[t]{0.45\linewidth}
        % \includegraphics[width=\linewidth]{figures/comparison/media_images_013.jpg}
        % \caption{\theprompt{A bat}}
        % \end{subfigure}
\\
        % \subfloat[]{
        %    \raisebox{0.75in}{\rotatebox[origin=t]{90}{{Baseline 2}}}
        % } 
        \subcaptionbox{\tiny{``An image composed of the repetition of a children's book illustration of a nerdy bear. There should be no gaps nor overlaps. The object is always the same in all repetitions.''}}[0.45\linewidth]{\includegraphics[width=\linewidth]{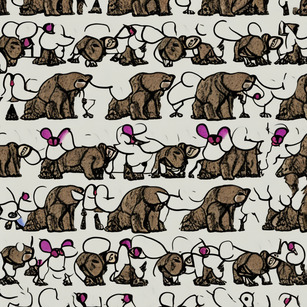}}
        % \hfill
        % \subcaptionbox{\tiny{``An Escher-like image of a penguin.''}}[0.45\linewidth]{\includegraphics[width=\linewidth]{figures/comparison/media_images_028.jpg}}
        % \hfill
        \subcaptionbox{\tiny{``An Escher pattern of a comic book illustration of Saturn with shooting stars.''}}[0.45\linewidth]{\includegraphics[width=\linewidth]{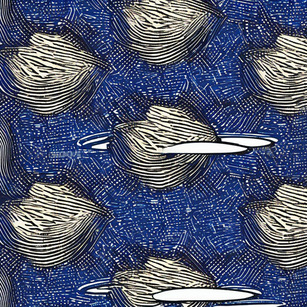}}
        % \hfill
        % \subcaptionbox{\tiny{``An image composed of the repetition of a lion, best quality, extremely detailed in the style of Escher. There should be no gaps nor overlaps.''}}[0.45\linewidth]{\includegraphics[width=\linewidth]{figures/comparison/media_images_075.jpg}}\hfill
        % \subcaptionbox{\tiny{``An Escher-like tiling of a bat.''}}[0.45\linewidth]{\includegraphics[width=\linewidth]{figures/comparison/media_images_167.jpg}}
        % \end{subfigure}
        % \begin{subfigure}[t]{0.45\linewidth}
        % \includegraphics[width=\linewidth]{figures/comparison/media_images_028.jpg}
        % % \subcaptionbox{\tiny{``An Escher-like image of a penguin.''}}[0.45\linewidth]
        % \end{subfigure}
        % \begin{subfigure}[t]{0.45\linewidth}
        % \includegraphics[width=\linewidth]{figures/comparison/media_images_043.jpg}
        % % \subcaptionbox{\tiny{``An Escher pattern of a comic book illustration of Saturn with shooting stars.''}}[0.45\linewidth]
        % \end{subfigure}
        % \begin{subfigure}[t]{0.45\linewidth}
        % \includegraphics[width=\linewidth]{figures/comparison/media_images_075.jpg}
        % % \subcaptionbox{\tiny{``An image composed of the repetition of a lion, best quality, extremely detailed in the style of Escher. There should be no gaps nor overlaps.''}}[0.45\linewidth]
        % \end{subfigure}
        % \begin{subfigure}[t]{0.45\linewidth}
        % \includegraphics[width=\linewidth]{figures/comparison/media_images_167.jpg}
        % % \subcaptionbox{\tiny{``An Escher-like tiling of a bat.''}}[0.45\linewidth]
        % \end{subfigure}
\captionsetup{justification=justified}
    \caption{\textbf{More baseline comparisons.} We compare our method (\textit{top row})  with two image-based baselines on five examples. The first baseline (\textit{middle row}) repeats an pixel image in a 5x5 grid and run random crops through SDS to fit a text prompt. Please see text for more details. The second baseline (\textit{bottom row}) shows our best attempt at “prompt-engineering” to encourage SD~\cite{stablediffusion} to generate a tiling. The best prompt is different for each sample and we show the prompt beneath the image. We report in supplementary all the prompts we tried. }
    \label{fig:comparison}
\end{figure}
